# Supplementary material for: Les Houches 2017: Physics at TeV Colliders Standard Model Working Group Report
Source: arXiv:1803.07977 source file (2018-03-21)

# $N_2^{(1)}$ (CMS-like): parton $\rightarrow$ hadron

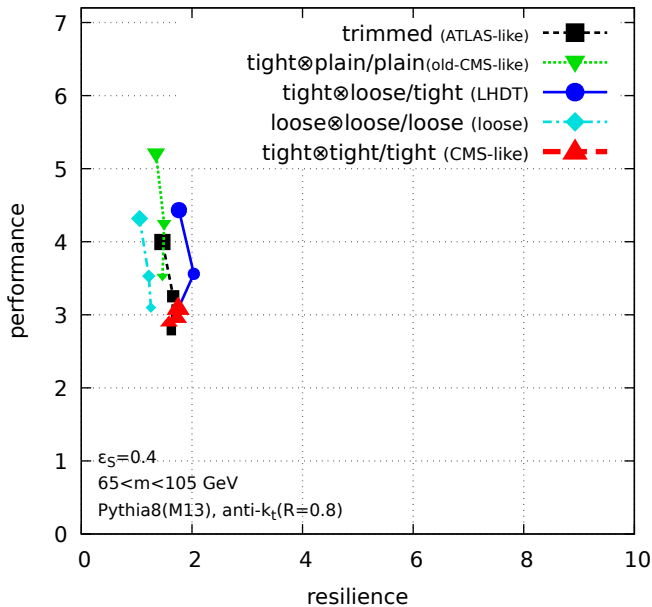

# $N_2^{(1)}$ (CMS-like): hadron $\rightarrow$ truth

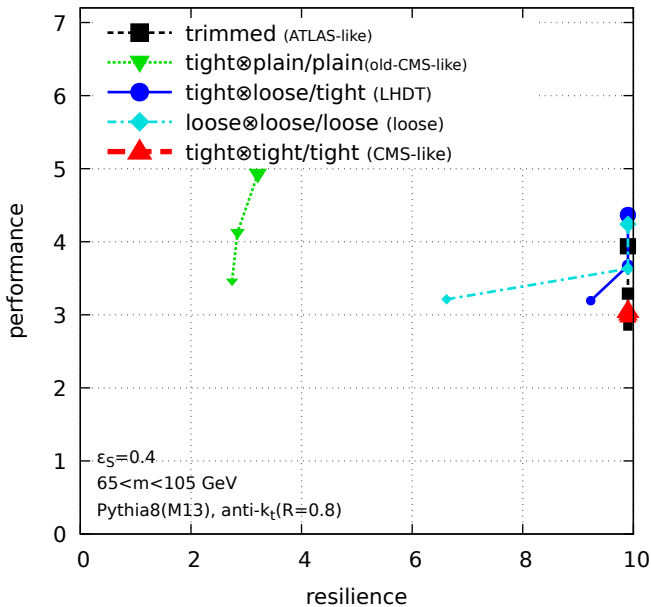

# $D_2^{(1)}$ (ATLAS-like): parton $\rightarrow$ hadron

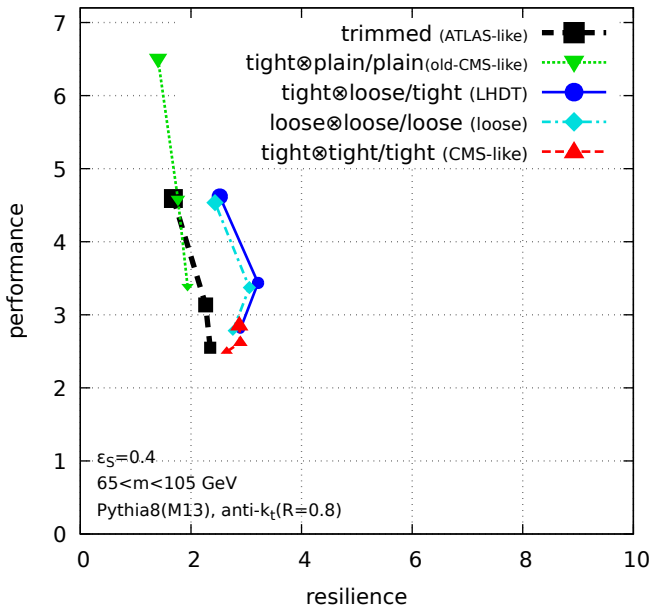

# $D_2^{(1)}$ (ATLAS-like): hadron $\rightarrow$ truth

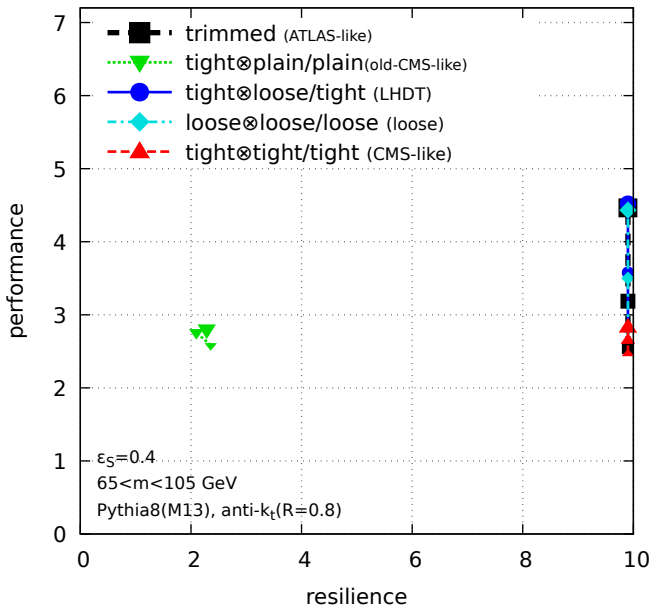

# $D_2^{(2)}$ (LHDT): parton $\rightarrow$ hadron

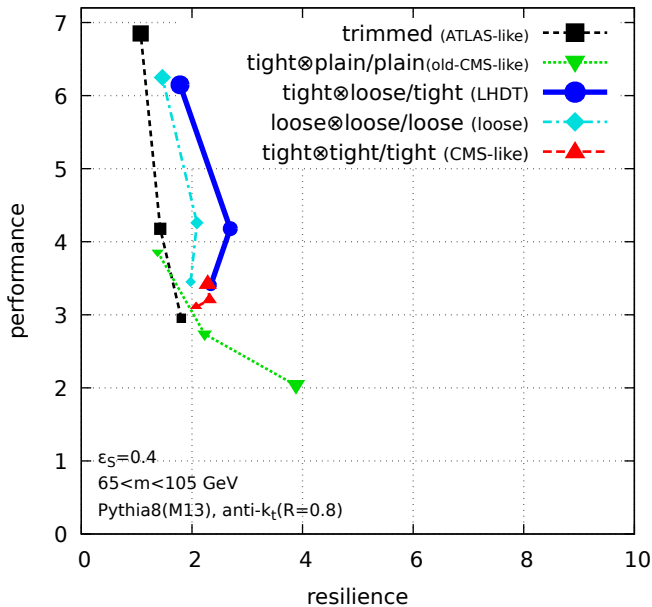

# $D_2^{(2)}$ (LHDT): hadron $\rightarrow$ truth

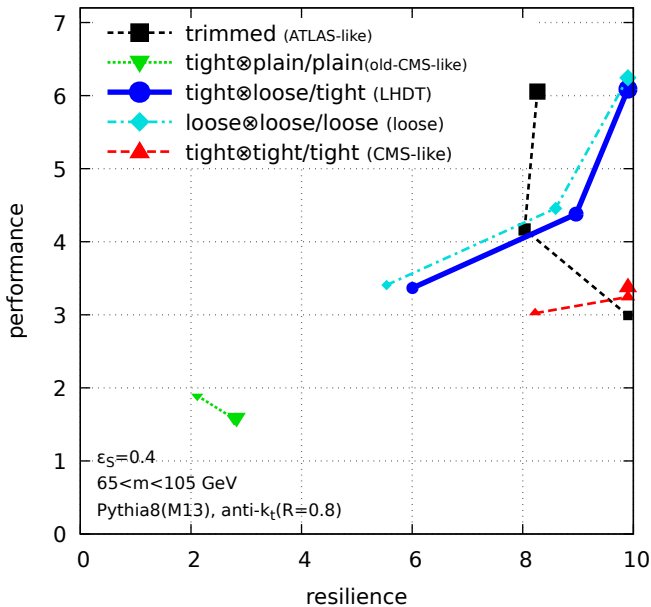

Supplement: Supplementary file 1 [file jetsub_2prong_grooming-scan.pdf]
