# Supplementary material for: Les Houches 2017: Physics at TeV Colliders Standard Model Working Group Report
Source: arXiv:1803.07977 source file (2018-03-21)

# ATLAS-like(trimmed) v. CMS-like (tight)

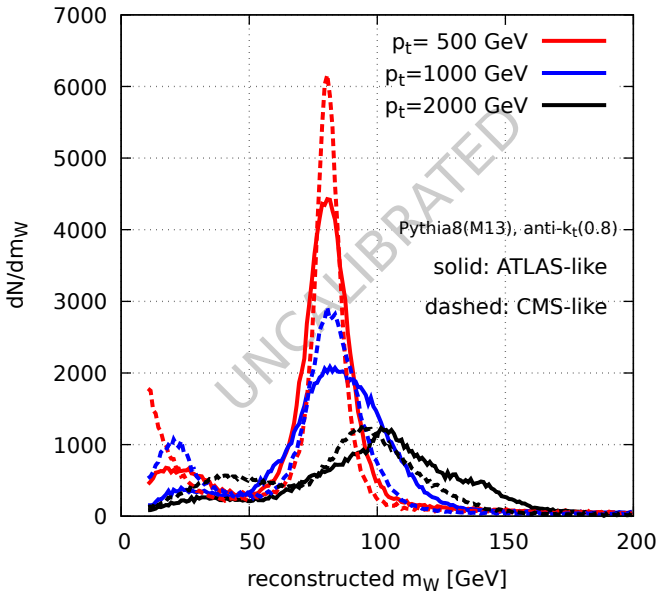

# ATLAS-like

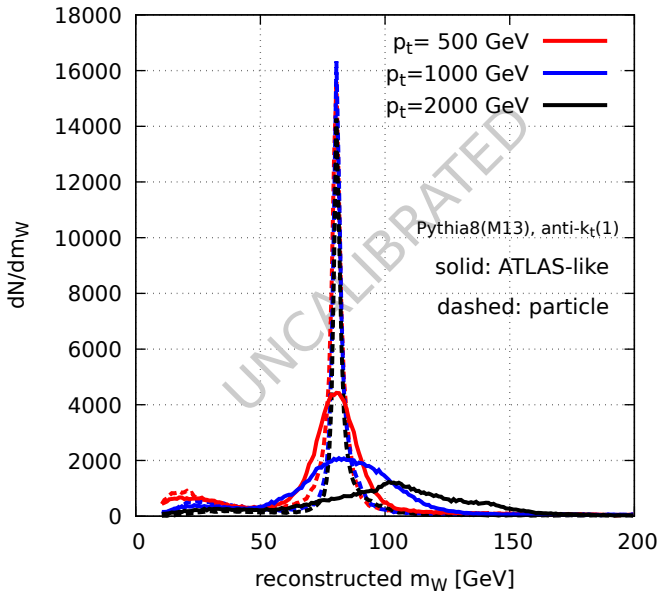

# CMS-like

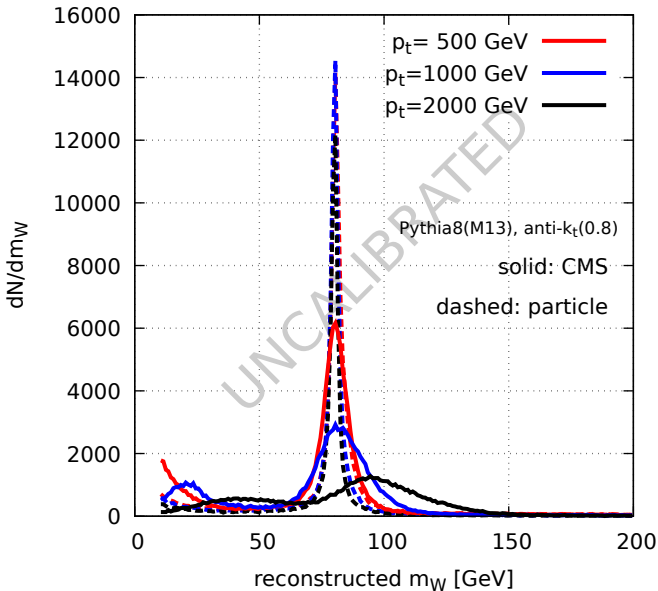

Supplement: Supplementary file 2 [file jetsub_2prong_mass-detector.pdf]
