# Supplementary material for: Les Houches 2017: Physics at TeV Colliders Standard Model Working Group Report
Source: arXiv:1803.07977 source file (2018-03-21)

# ATLAS-like (particle v. parton)

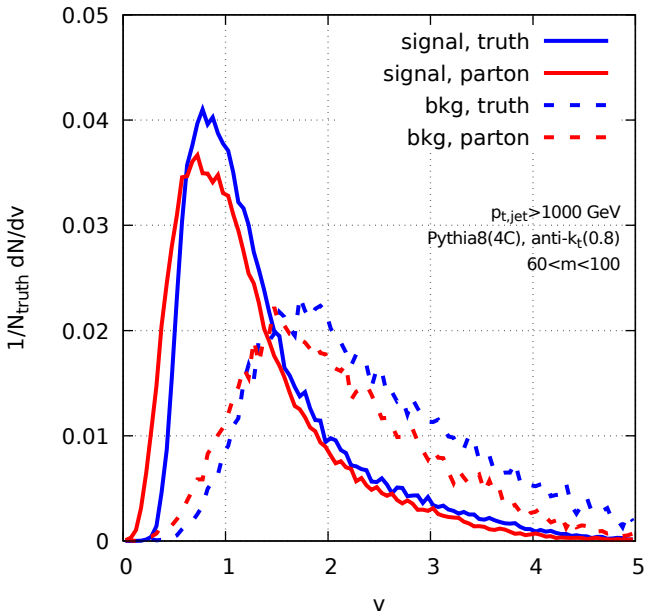

# CMS-like (particle v. parton)

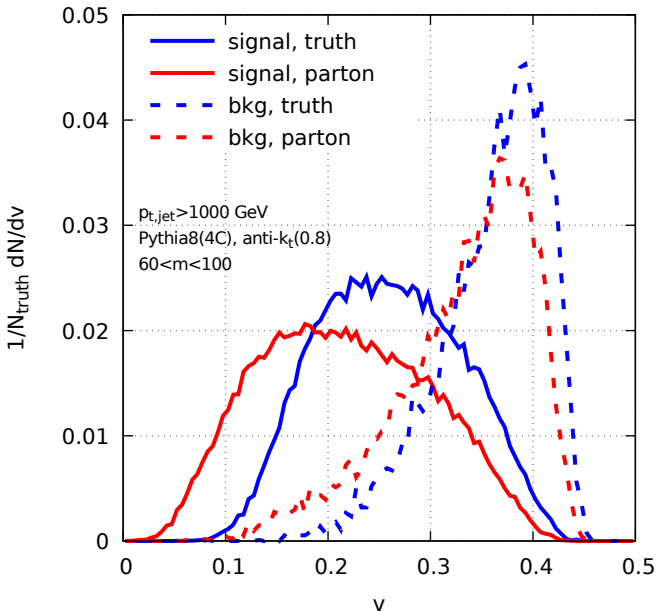

# resilience-oriented (particle v. parton)

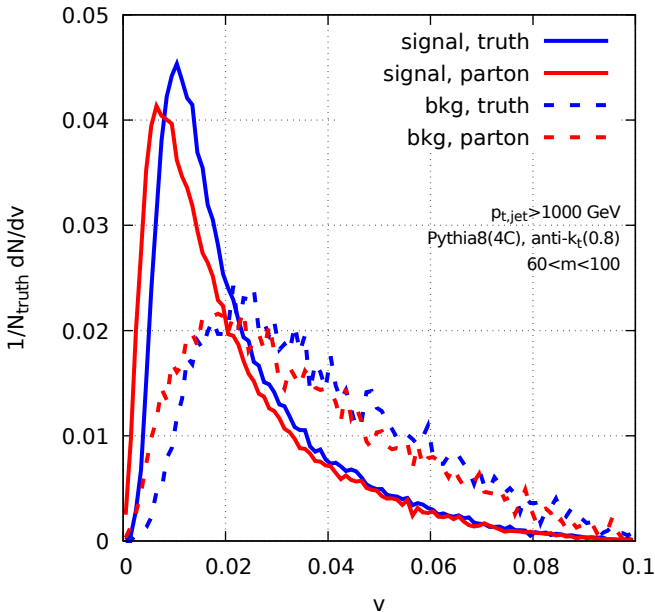

# performance-oriented (particle v. parton)

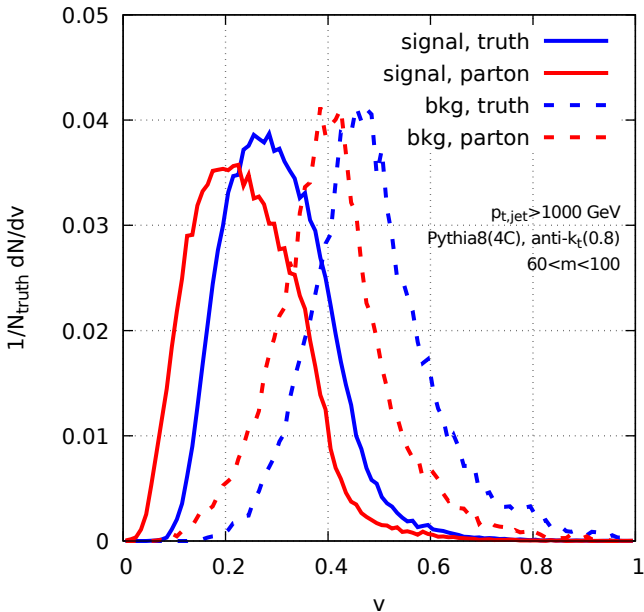

Supplement: Supplementary file 3 [file jetsub_2prong_shape-distribs-R0.8.pdf]
