# Supplementary material for: Les Houches 2017: Physics at TeV Colliders Standard Model Working Group Report
Source: arXiv:1803.07977 source file (2018-03-21)

# ATLAS-like [ $D_2^{(1)}$ (trim)]

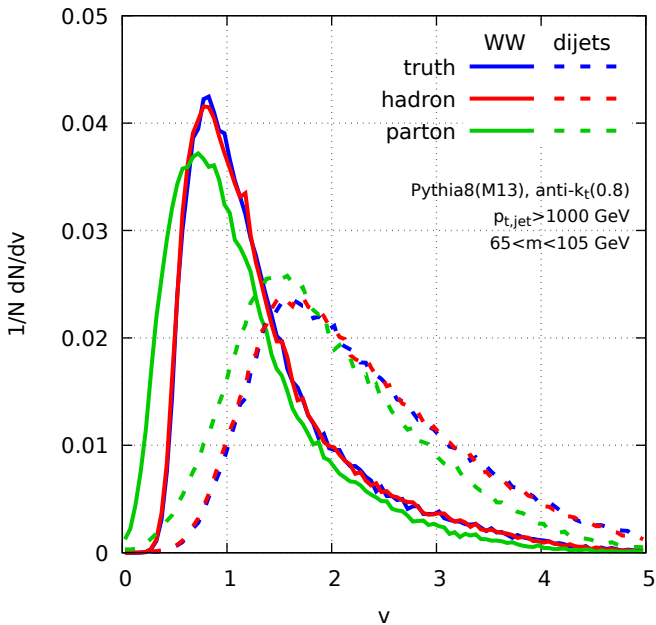

# CMS-like $[N_2^{(1)}(t \otimes t/t)]$

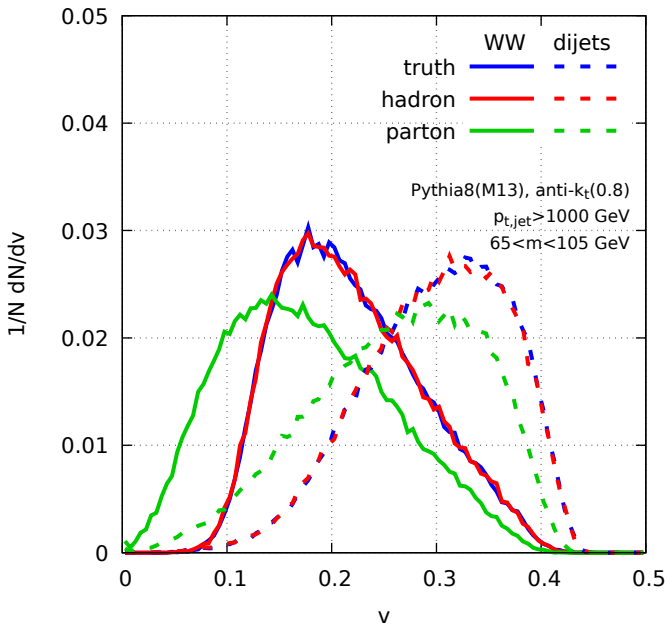

LHDT  $[D_2^{(2)}(t \otimes I/t)]$

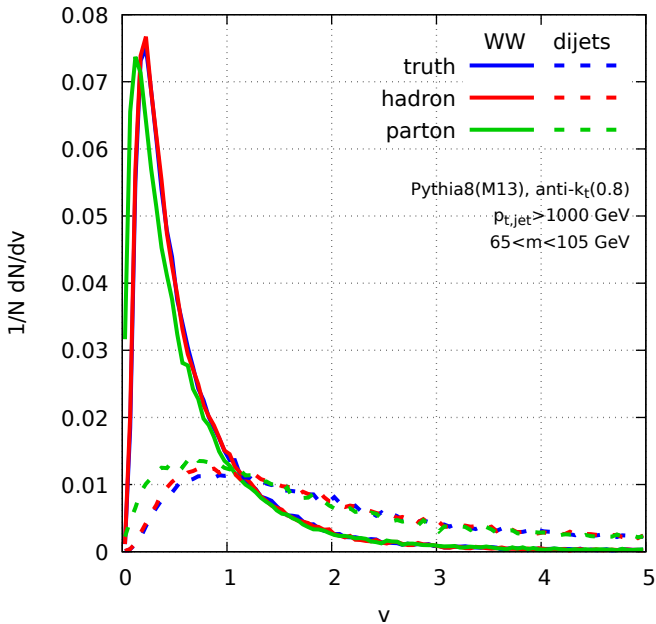

Supplement: Supplementary file 5 [file jetsub_2prong_shape-distribs.pdf]
