# Supplementary material for: Les Houches 2017: Physics at TeV Colliders Standard Model Working Group Report
Source: arXiv:1803.07977 source file (2018-03-21)

# tight $\otimes$ loose/tight(LHDT): parton $\rightarrow$ hadron

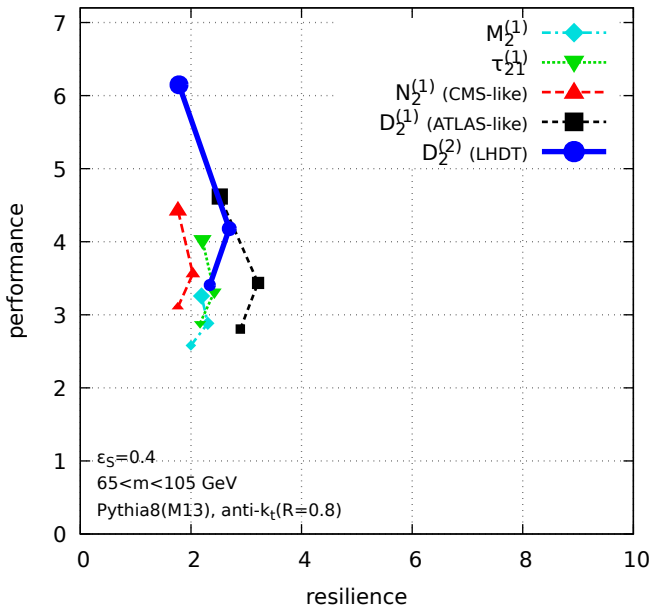

# tight $\otimes$ loose/tight(LHDT): hadron $\rightarrow$ truth

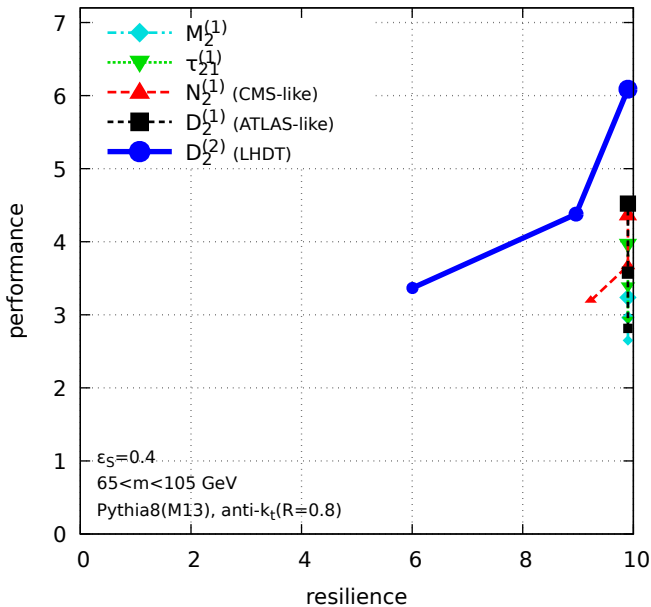

# tight $\otimes$ tight/tight(CMS-like): parton $\rightarrow$ hadron

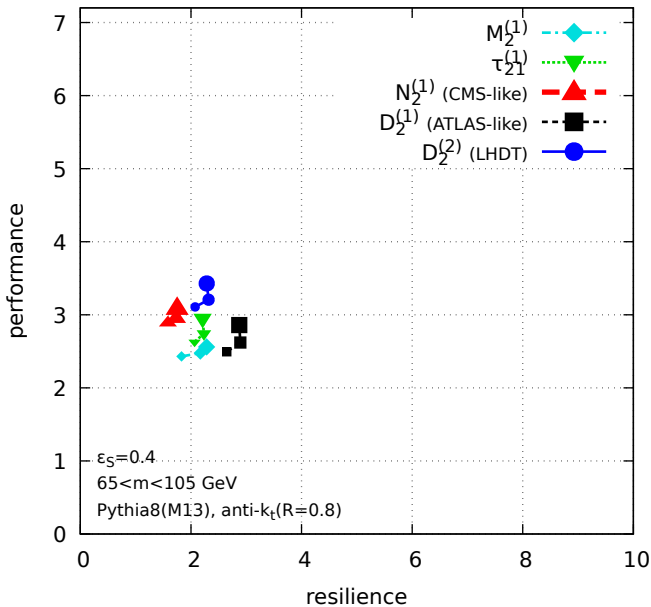

# tight $\otimes$ tight/tight(CMS-like): hadron $\rightarrow$ truth

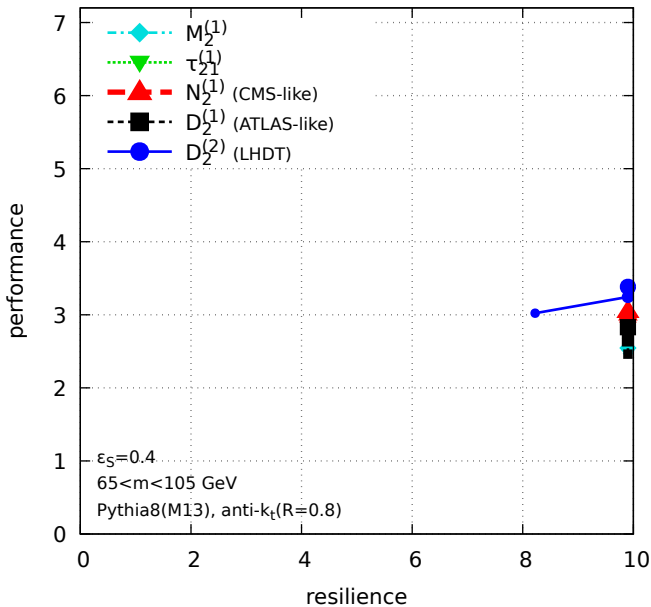

# trimmed (ATLAS-like): parton $\rightarrow$ hadron

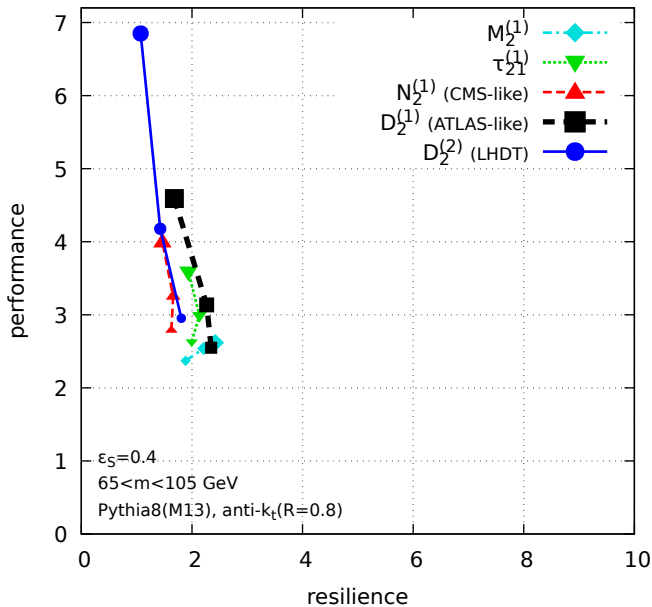

# trimmed (ATLAS-like): hadron $\rightarrow$ truth

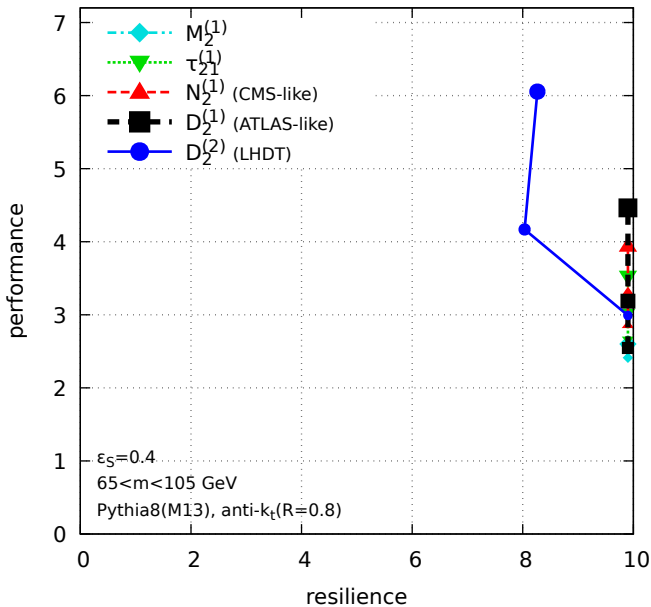

Supplement: Supplementary file 6 [file jetsub_2prong_shape-scan.pdf]
